# Supplementary material for: EP-PINNs: Cardiac Electrophysiology Characterisation using Physics-Informed Neural Networks
Source: arXiv:2112.07703 source file (2021-12-14)
Supplement: Supplementary file 1 [file EP-PINNsPaper_SupplementaryInfo_AfterReview2.pdf]

## Supplementary Tables

| Parameter                    | Value Used               | Additional Values        |
|------------------------------|--------------------------|--------------------------|
| <b>a</b>                     | 0.010                    | 0.002                    |
| <b>b</b>                     | 0.150                    | 0.075                    |
| <b><math>\epsilon</math></b> | 0.002                    | -                        |
| <b>k</b>                     | 8.00                     | -                        |
| <b><math>\mu_1</math></b>    | 0.20                     | -                        |
| <b><math>\mu_2</math></b>    | 0.30                     | -                        |
| <b>D</b>                     | 0.10 mm <sup>2</sup> /TU | 0.02 mm <sup>2</sup> /TU |

*Supplementary Table 1 - Values used for model parameters in the monodomain Aliev Panfilov model, from (Göktepe and Kuhl, 2009; Nash and Panfilov, 2004). All variables are in consistent arbitrary units (AU), except D. TU: time units. The values in the 3<sup>rd</sup> column were used in additional tests to test EP-PINNs performance with different parameters.*

|                             | EP-PINNs Architecture    | Training Scheme                                                                                                     | Typical Training Time | Train, Test Data Split (% , #points)                         |
|-----------------------------|--------------------------|---------------------------------------------------------------------------------------------------------------------|-----------------------|--------------------------------------------------------------|
| <b>1D</b>                   | A: 4 layers x 32 neurons | 1                                                                                                                   | 25 min                | 10% ( $1.40 \times 10^2$ pts), 90% ( $1.26 \times 10^3$ pts) |
| <b>2D Homogeneous</b>       |                          |                                                                                                                     |                       |                                                              |
| Planar or Centrifugal Wave  | A: 4 layers x 32 neurons | 2<br>$\text{iter}_1 = 1.5 \times 10^4$ ;<br>$\text{lr}_2 = 5 \times 10^{-4}$ ;<br>$\text{iter}_2 = 1.2 \times 10^5$ | 2.5 h                 | 20% ( $1.40 \times 10^5$ pts), 80% ( $5.60 \times 10^5$ pts) |
| Spiral Wave                 | A: 5 layers x 60 neurons | 2<br>$\text{iter}_1 = 1.5 \times 10^4$ ;<br>$\text{lr}_2 = 10^{-4}$ ; $\text{iter}_2 = 1.5 \times 10^5$             | 7 h                   |                                                              |
| <b>2D Heterogeneous</b>     |                          |                                                                                                                     |                       |                                                              |
| Centrifugal Wave            | B: 4 layers x 32 neurons | 2<br>$\text{iter}_1 = 1.5 \times 10^4$ ;<br>$\text{lr}_2 = 5 \times 10^{-4}$ ;<br>$\text{iter}_2 = 1.2 \times 10^5$ | 7 h                   | 20% ( $1.40 \times 10^5$ pts), 80% ( $5.60 \times 10^5$ pts) |
| Spiral Wave                 | B: 5 layers x 60 neurons | 2<br>$\text{iter}_1 = 1.5 \times 10^4$ ;<br>$\text{lr}_2 = 10^{-4}$ ; $\text{iter}_2 = 1.5 \times 10^5$             | 16 h                  |                                                              |
| <b>Canine Atrial Model</b>  | 4 layers x 32 neurons    | 1                                                                                                                   | 15 min                | 10% ( $1.40 \times 10^3$ pts), 90% ( $1.26 \times 10^3$ pts) |
| <b>Optical Mapping Data</b> | A: 6 layers x 60 neurons | 2<br>$\text{iter}_1 = 5 \times 10^3$ ;<br>$\text{lr}_2 = 10^{-5}$ ; $\text{iter}_2 = 1.5 \times 10^5$               | 15 min                | 80% (116-200 pts), 20% (29-50 pts)                           |

*Supplementary Table 2 – Details of the network architecture, training schemes and typical training times used in the applications listed in this study. Details of architectures A and B and training schemes 1 and 2 can be found in Figure 2. The same settings were used for forward and inverse modes of EP-PINNs. In architecture B, the same number of layers and neurons is used in NN and NN\_D.*

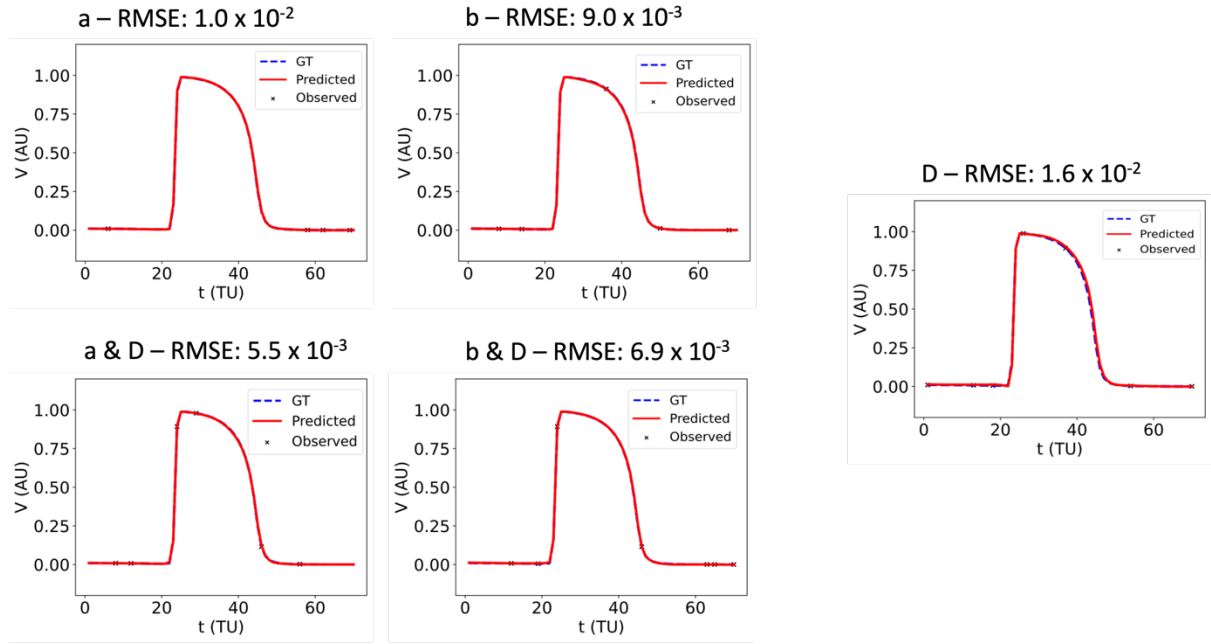

*Supplementary Figure 1 – Representative action potentials in the 1D inverse scenario, for estimates of parameters: a (top left), b (top right), a & D (bottom left), b & D (bottom right) and D (far right). The total RMSE for  $V$  estimates (in AU) for each case is also shown.*

## References

- Göktepe, S., and Kuhl, E. (2009). Electromechanics of the heart: a unified approach to the strongly coupled excitation–contraction problem. *Comput. Mech.* 45, 227–243.  
doi:10.1007/s00466-009-0434-z.
- Nash, M. P., and Panfilov, A. (2004). Electromechanical model of excitable tissue to study reentrant cardiac arrhythmias. *Prog. Biophys. Mol. Biol.* 85, 501–522.  
doi:10.1016/J.PBIOMOLBIO.2004.01.016.
